# Supplementary material for: From Average Effects to Targeted Assignment: A Causal Machine Learning Analysis of Swiss Active Labor Market Policies
Source: arXiv:2410.23322 source file (2025-05-11)
Supplement: Supplementary file 1 [file gateb_appendix.tex]

\begin{figure}[H]
\captionsetup{font=small}  % Set the font size to "large"
\caption{Differences of GATEs to ATE of the Temporary Earnings with respect to non participants to programs for Temporary Work Permit sample}
% Education
\begin{minipage}[t]{0.55\textwidth}
 \includegraphics[width=0.80\textwidth]{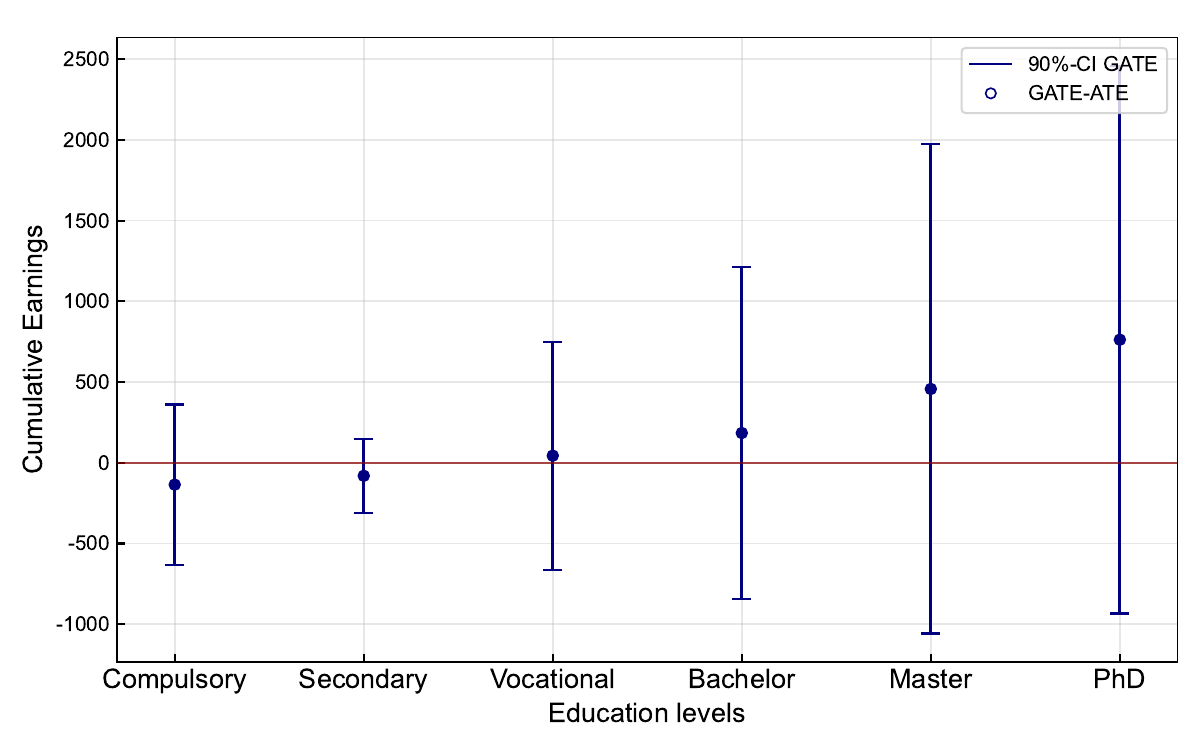}
	\end{minipage}
        \begin{minipage}[t]{0.55\textwidth}
 \includegraphics[width=0.80\textwidth]{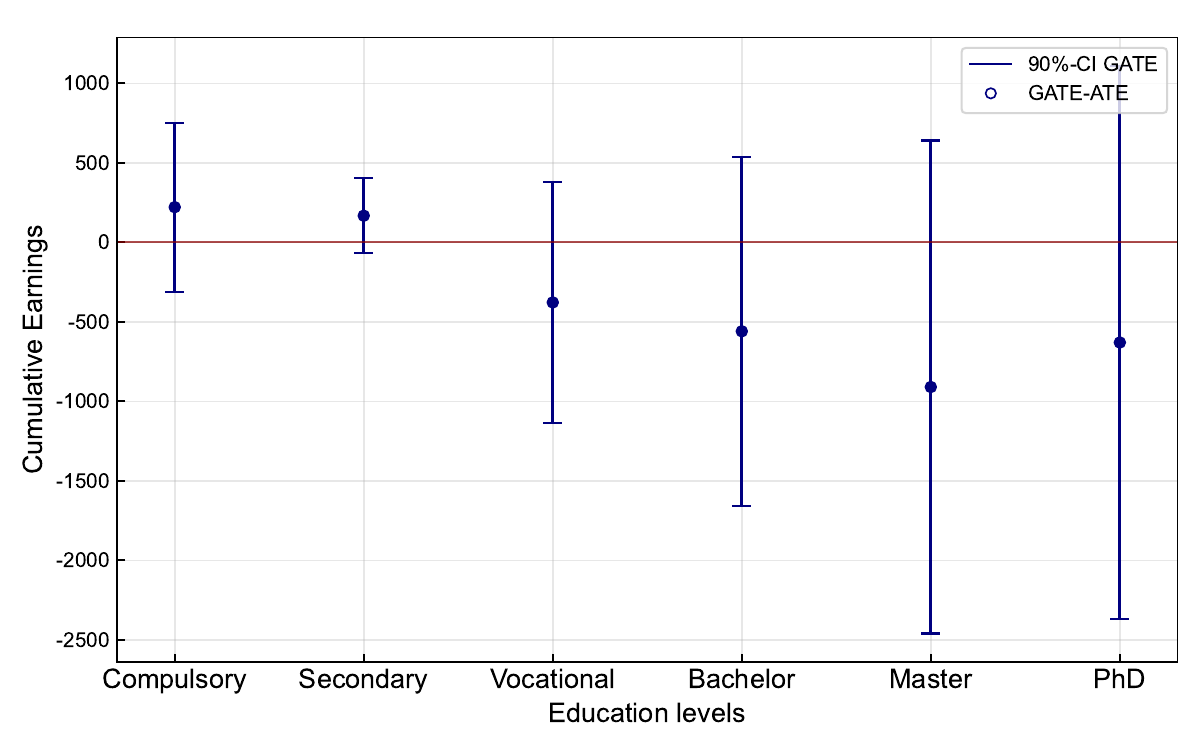}
	\end{minipage}
\begin{minipage}[t]{0.55\textwidth}
 \includegraphics[width=0.80\textwidth]{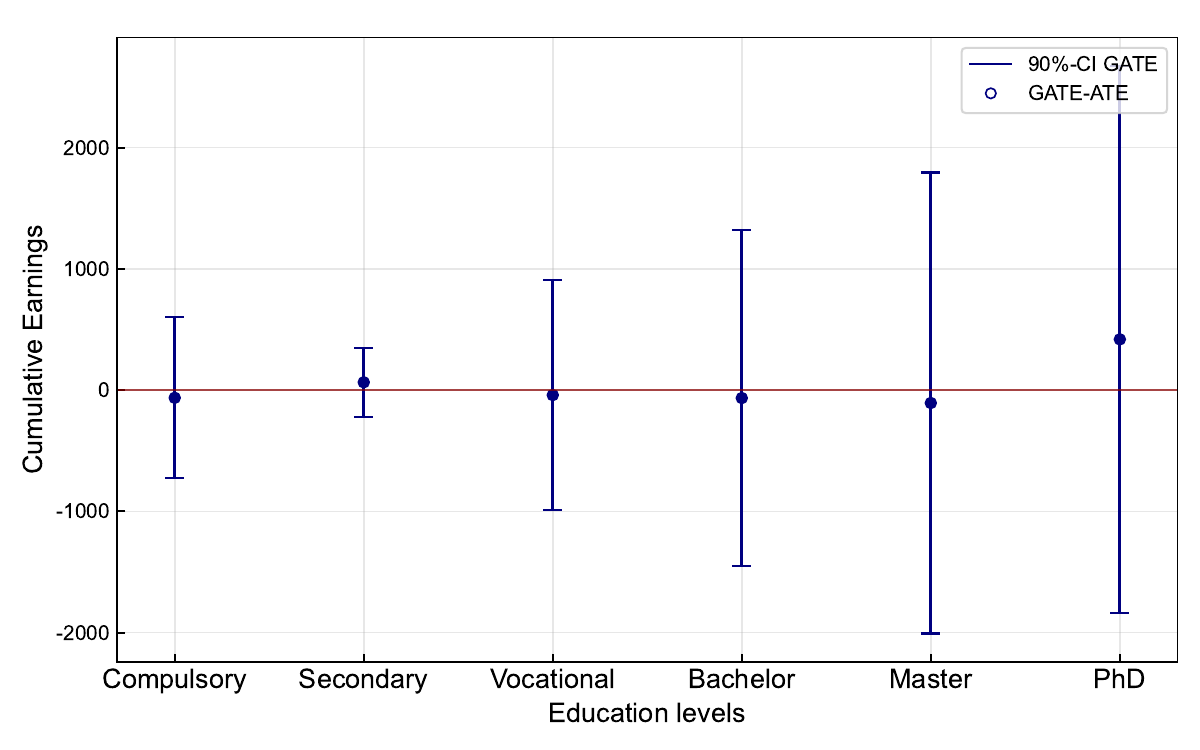}
	\end{minipage}
        \begin{minipage}[t]{0.55\textwidth}
 \includegraphics[width=0.80\textwidth]{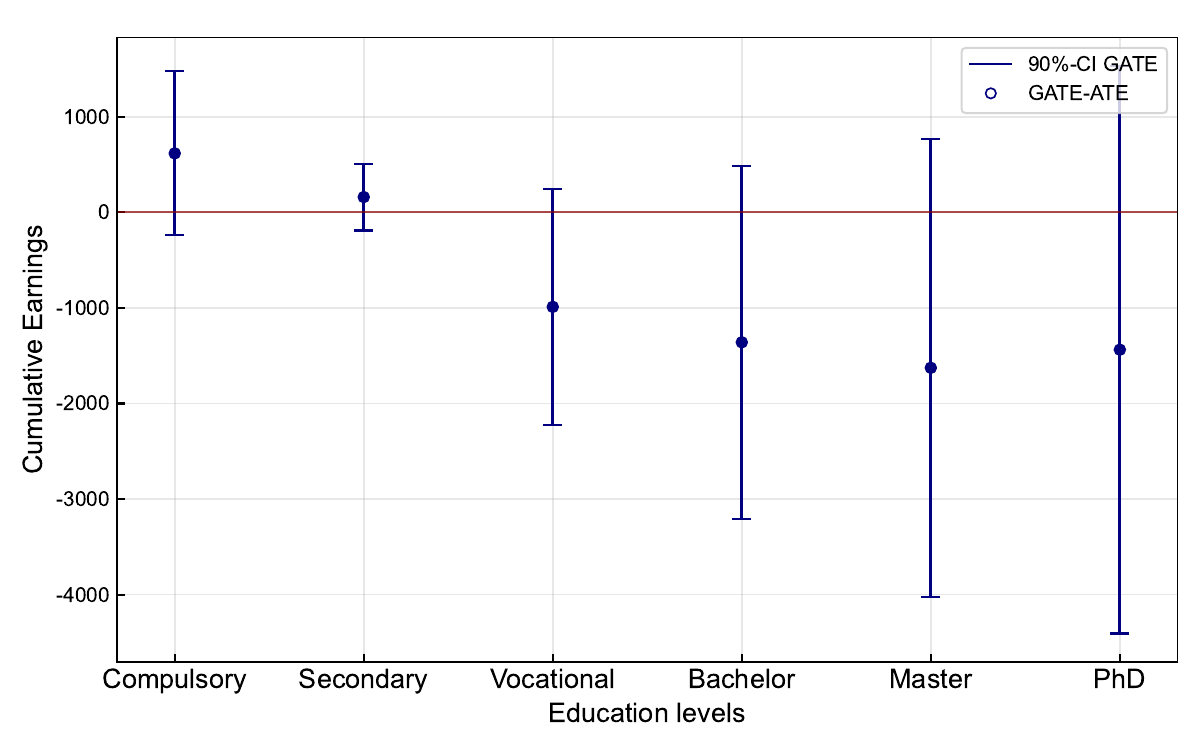}
	\end{minipage}
% Kindship
\begin{minipage}[t]{0.55\textwidth}
 \includegraphics[width=0.80\textwidth]{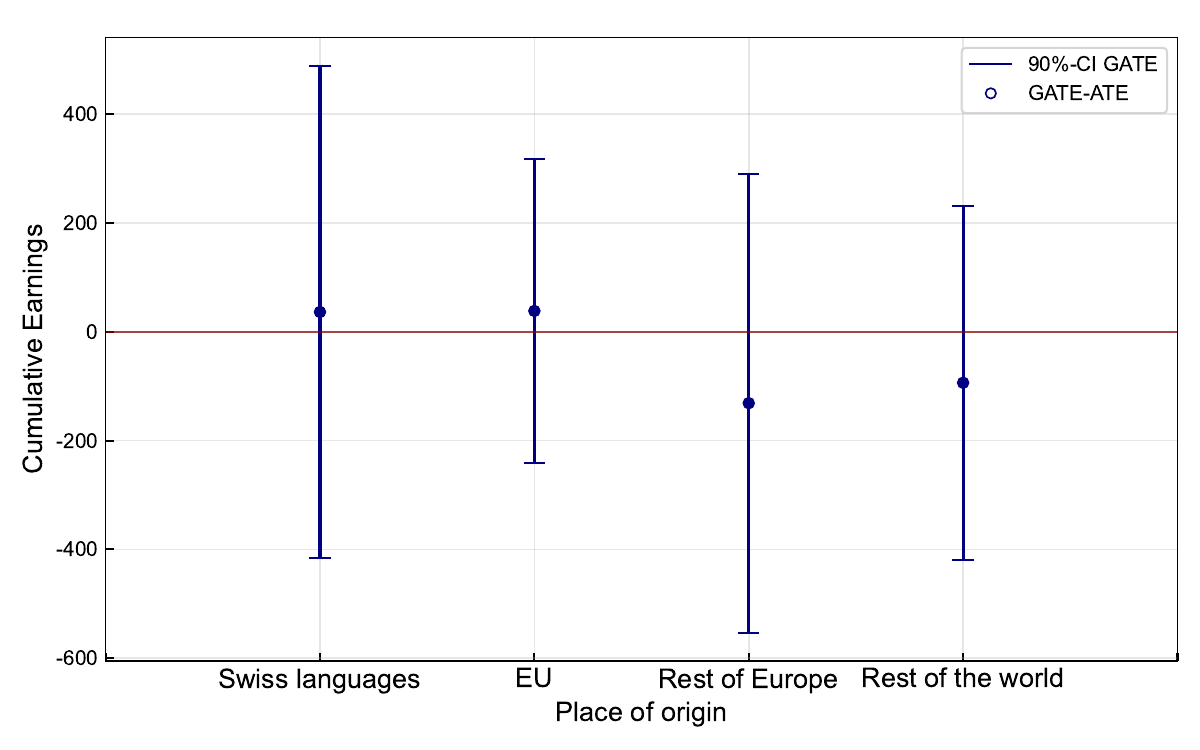}
	\end{minipage}
        \begin{minipage}[t]{0.55\textwidth}
 \includegraphics[width=0.80\textwidth]{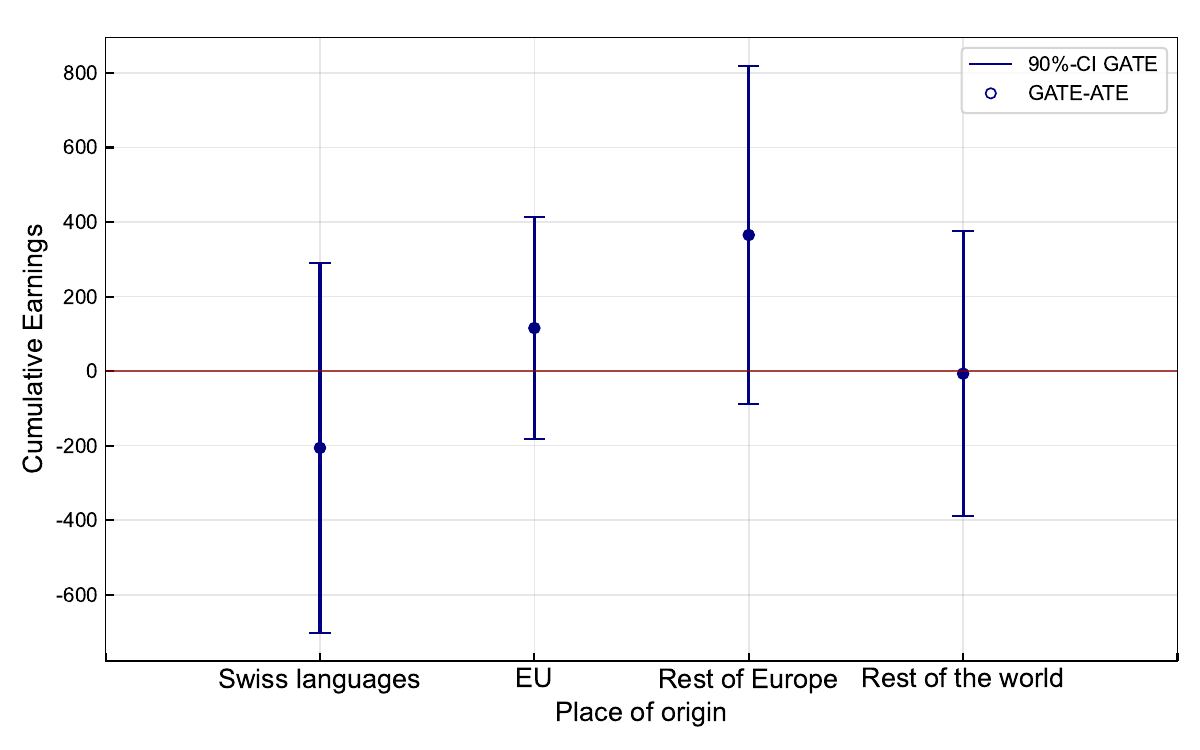}
	\end{minipage}
\begin{minipage}[t]{0.55\textwidth}
 \includegraphics[width=0.80\textwidth]{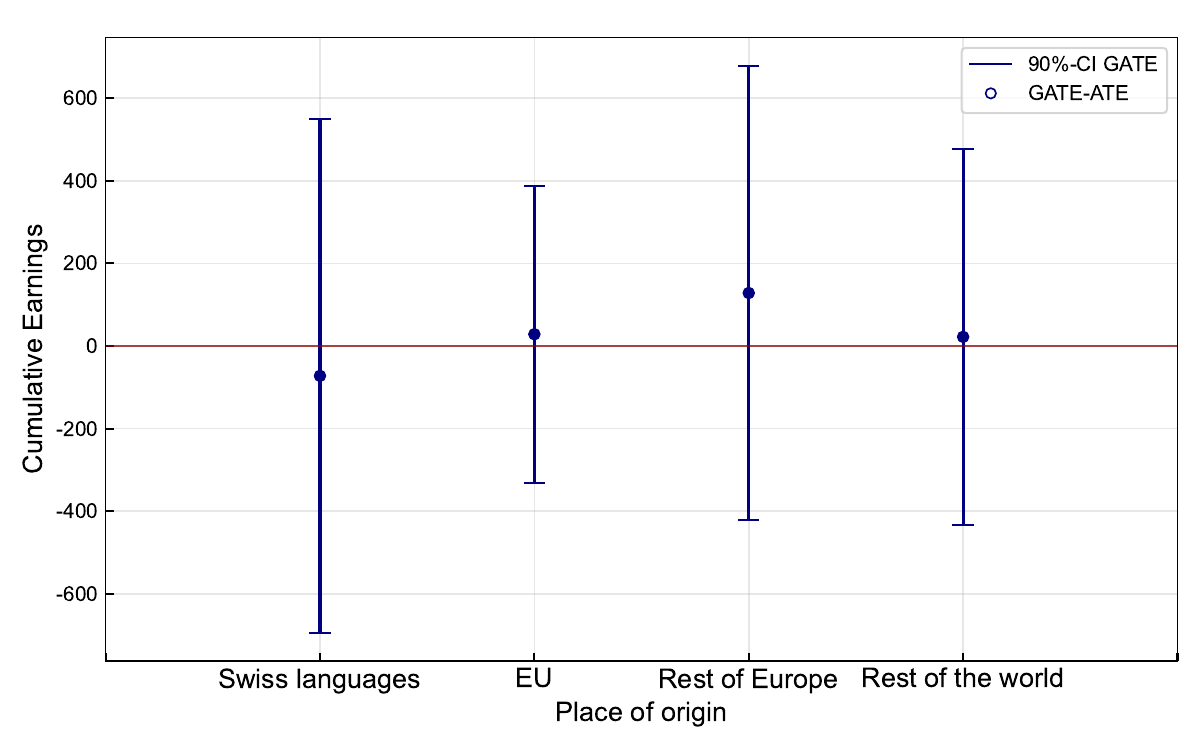}
	\end{minipage}
        \begin{minipage}[t]{0.55\textwidth}
 \includegraphics[width=0.80\textwidth]{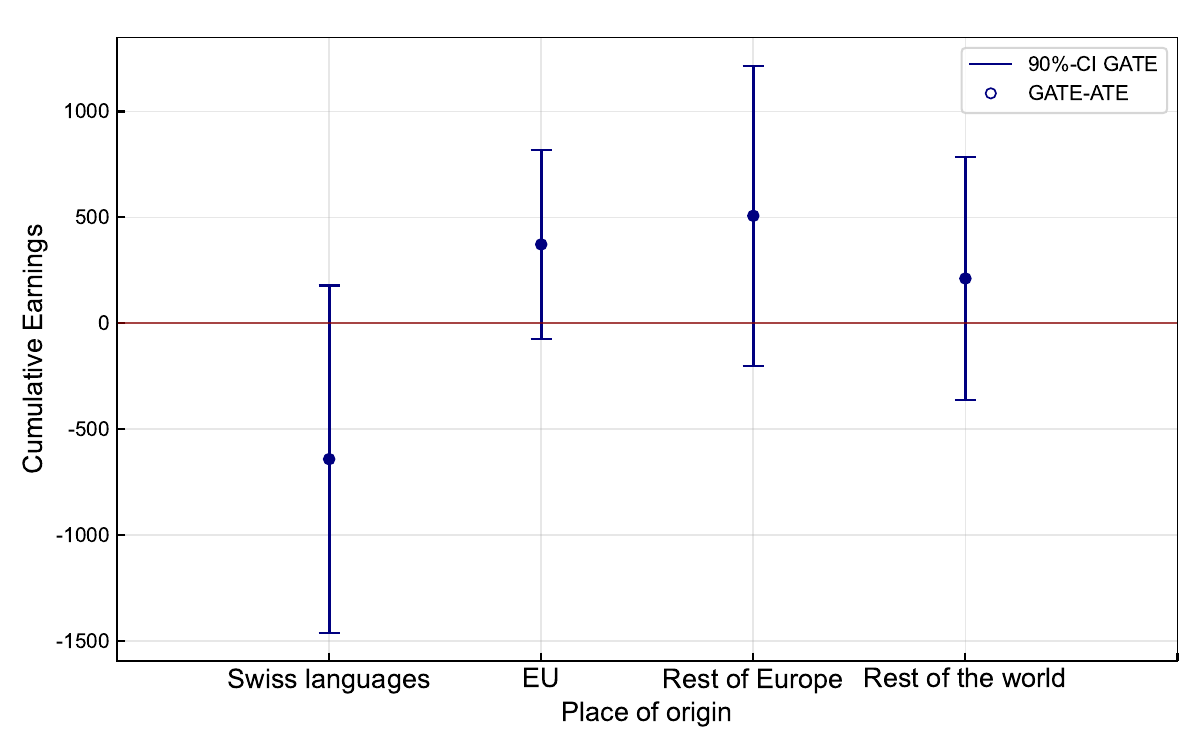}
	\end{minipage}
\caption*{\textit{Note:} The vertical axes measures the difference of GATEs to the ATE of different programs with respect to non participants and the 90\% confidence interval. On the horizontal axes the region of origin. The outcome is the cumulative earnings in the third year after the program start. Temporary Earnings: Upper-LHS, Basic Course: Upper-RHS, Technical course: Bottom-LHS, Temporary Employment: Bottom-RHS. }
\label{fig:gates_appendix}
\end{figure}

\begin{figure}[H]
\captionsetup{font=small}  % Set the font size to "large"
\caption{Differences of GATEs to ATE of the programmes with respect to non participants to programs for Temporary Work Permit sample.
Z-value: Proficiency in the local language}
\begin{minipage}[t]{0.55\textwidth}
 \includegraphics[width=0.80\textwidth]{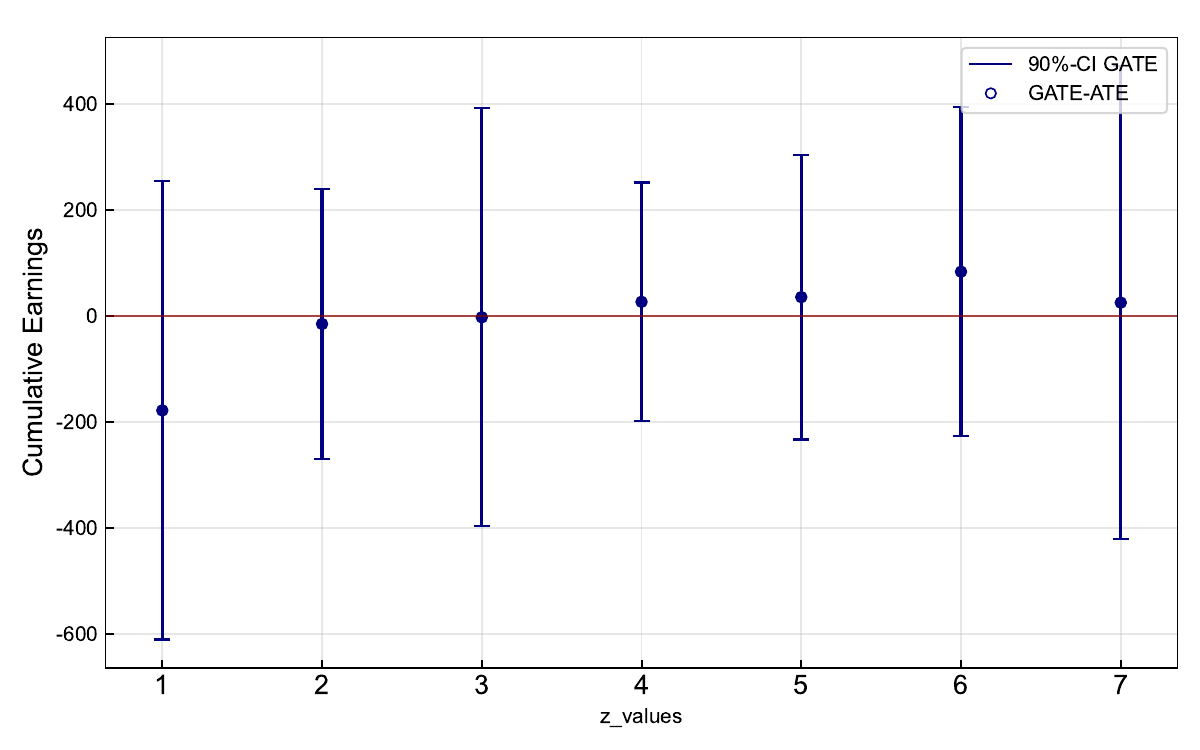}
	\end{minipage}
        \begin{minipage}[t]{0.55\textwidth}
 \includegraphics[width=0.80\textwidth]{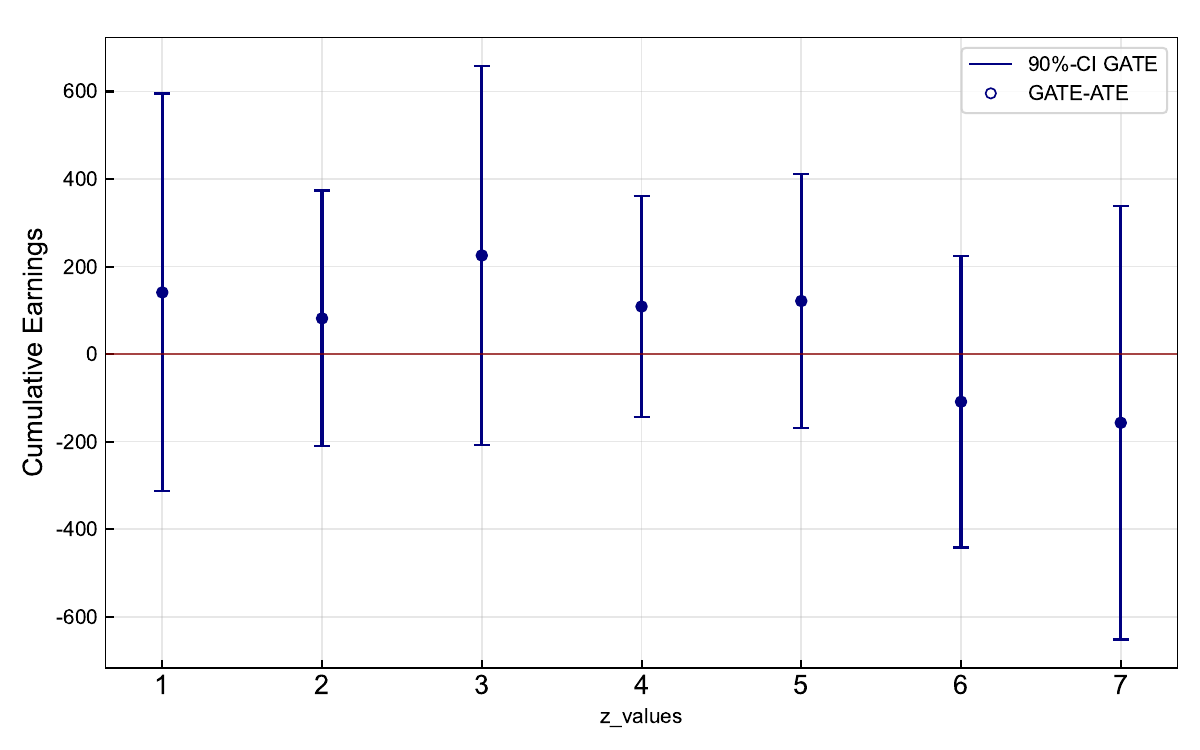}
	\end{minipage}
\begin{minipage}[t]{0.55\textwidth}
 \includegraphics[width=0.80\textwidth]{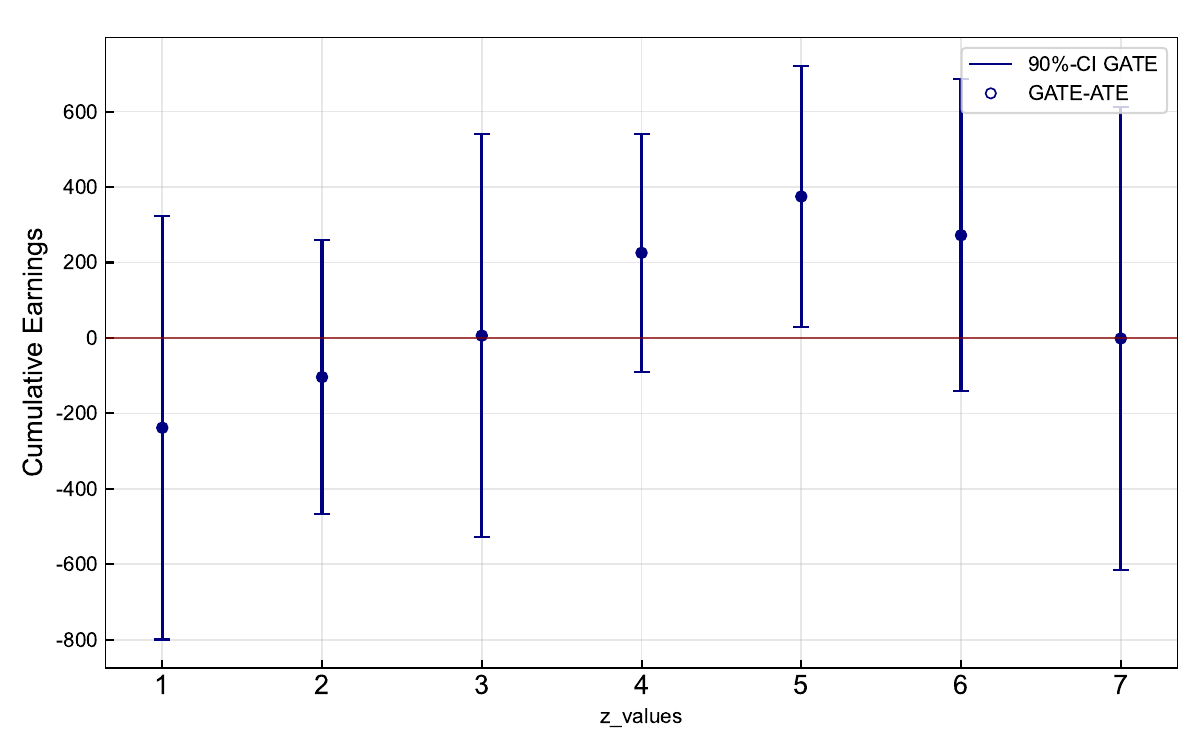}
	\end{minipage}
        \begin{minipage}[t]{0.55\textwidth}
 \includegraphics[width=0.80\textwidth]{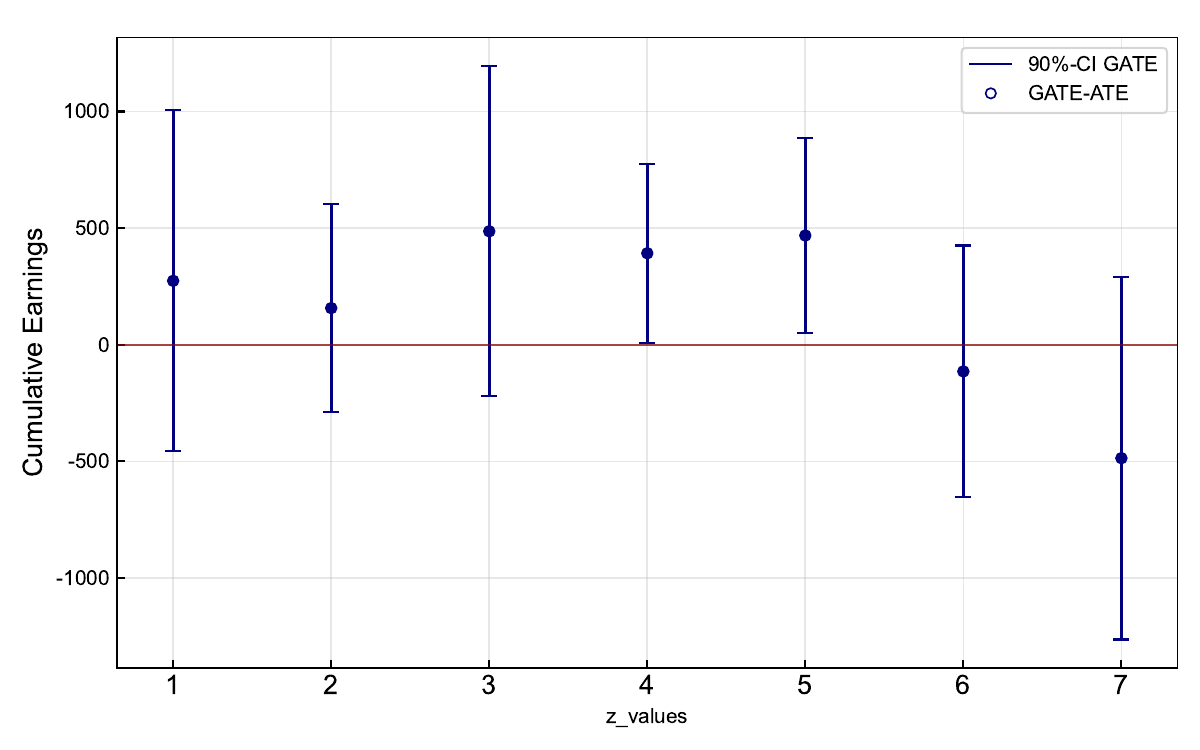}
	\end{minipage}
\caption*{\textit{Note:} The vertical axes measures the difference of GATEs to the ATE of different programs with respect to non participants and the 90\% confidence interval. On the horizontal axes the region of origin. The outcome is the cumulative earnings in the third year after the program start. Temporary Earnings: Upper-LHS, Basic Course: Upper-RHS, Technical course: Bottom-LHS, Temporary Employment: Bottom-RHS. }
\label{fig:gates_appendix}
\end{figure}
