# Supplementary material for: From Average Effects to Targeted Assignment: A Causal Machine Learning Analysis of Swiss Active Labor Market Policies
Source: arXiv:2410.23322 source file (2025-05-11)
Supplement: Supplementary file 2 [file gates_app.tex]

% GATEs app 
\begin{figure}[H]
\begin{minipage}[t]{0.55\textwidth}
 \includegraphics[width=0.80\textwidth]{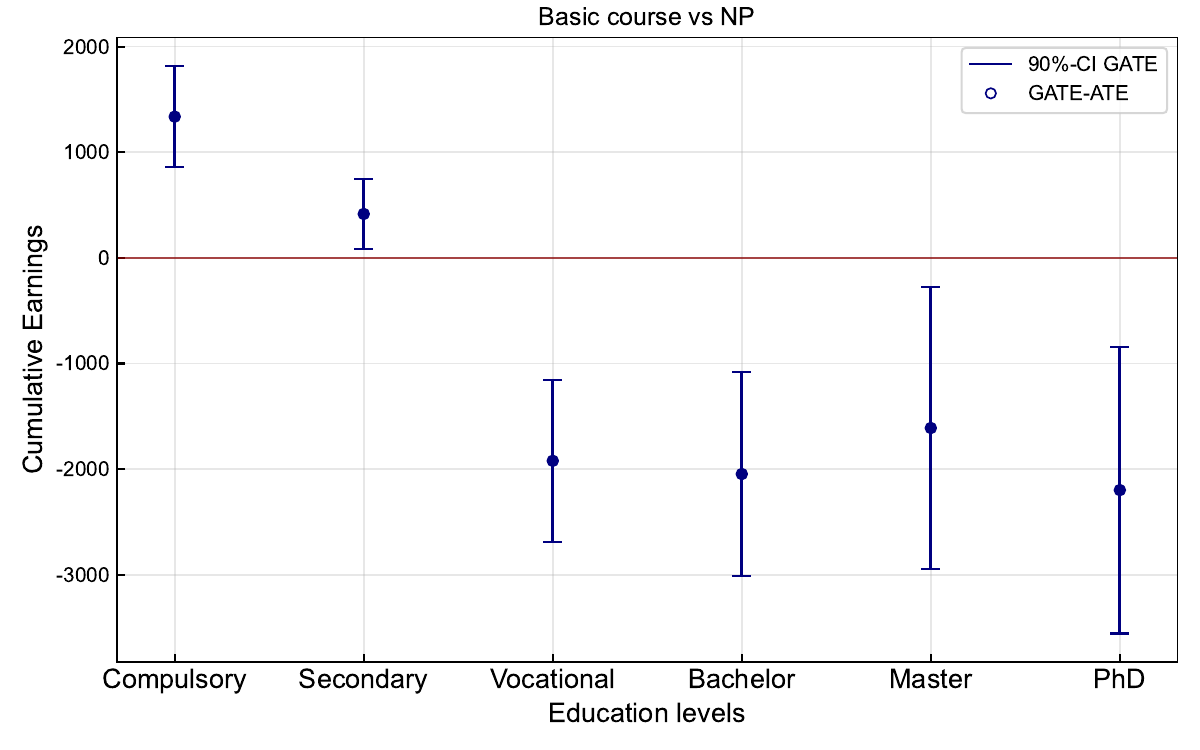}
	\end{minipage}
\begin{minipage}[t]{0.55\textwidth}
 \includegraphics[width=0.80\textwidth]{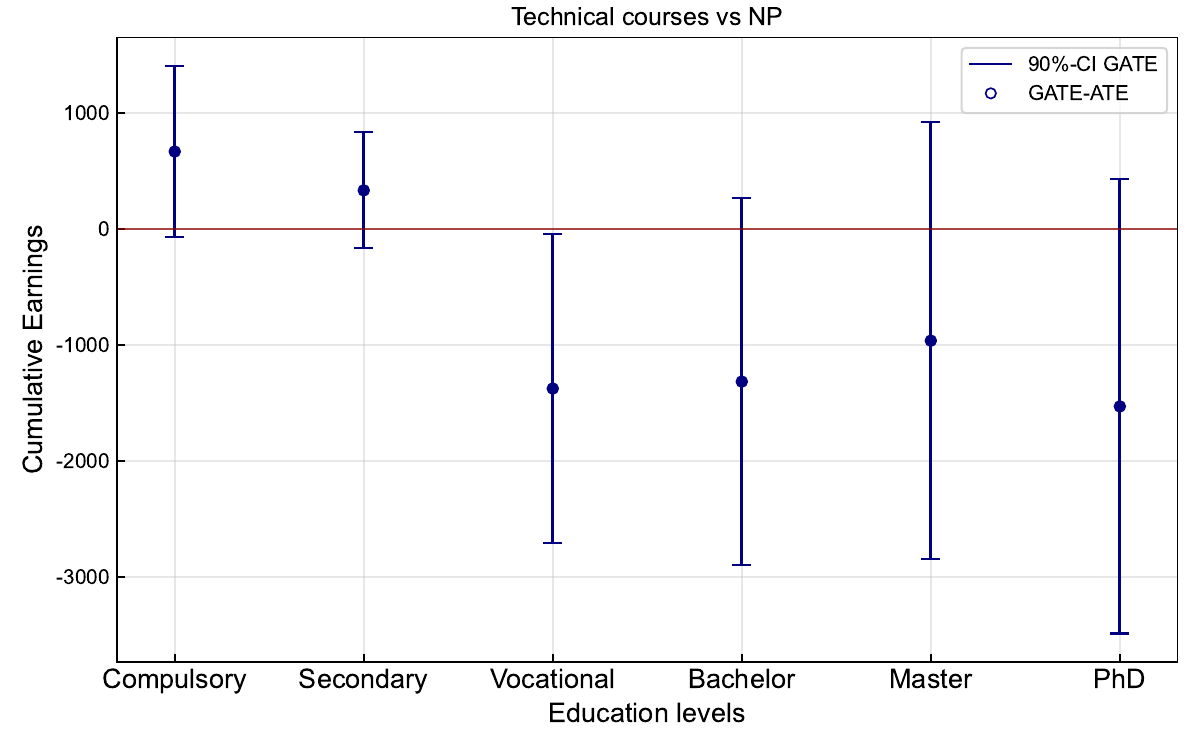}
	\end{minipage}
\begin{minipage}[t]{0.55\textwidth}
 \includegraphics[width=0.80\textwidth]{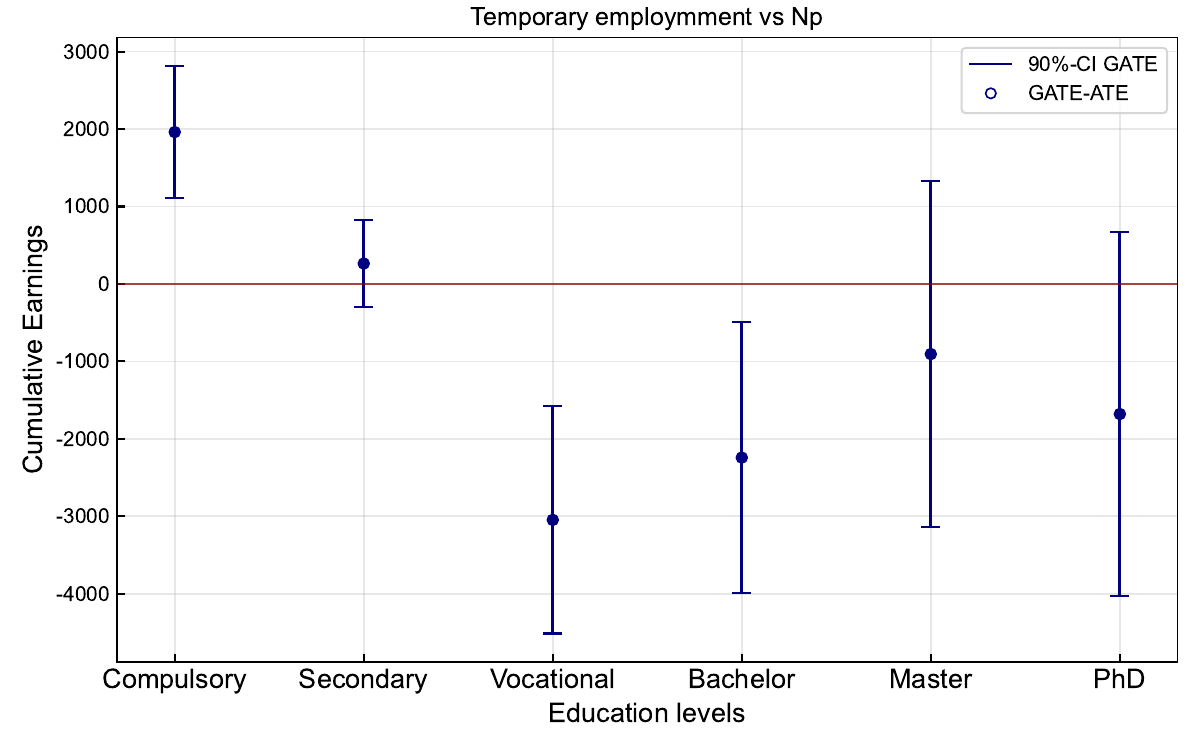}
\end{minipage}
% Proficiency
 \begin{minipage}[t]{0.55\textwidth}
 \includegraphics[width=0.80\textwidth]{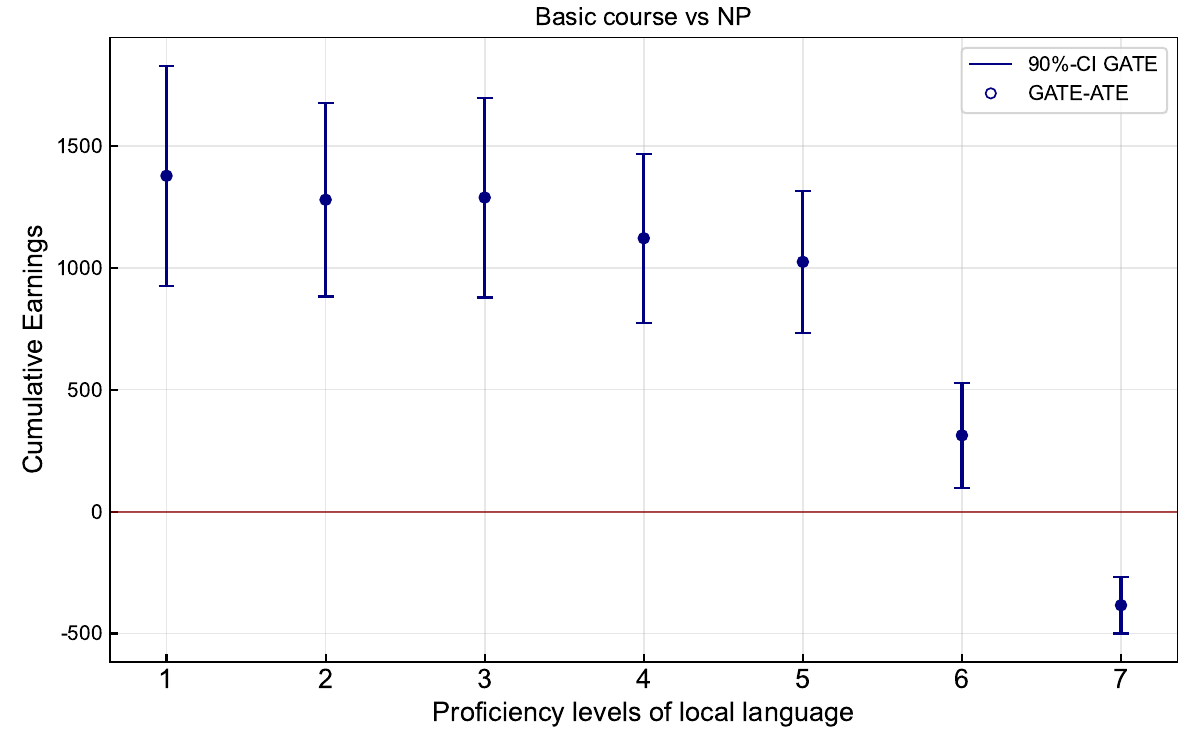}
	\end{minipage}
  \begin{minipage}[t]{0.55\textwidth}
 \includegraphics[width=0.80\textwidth]{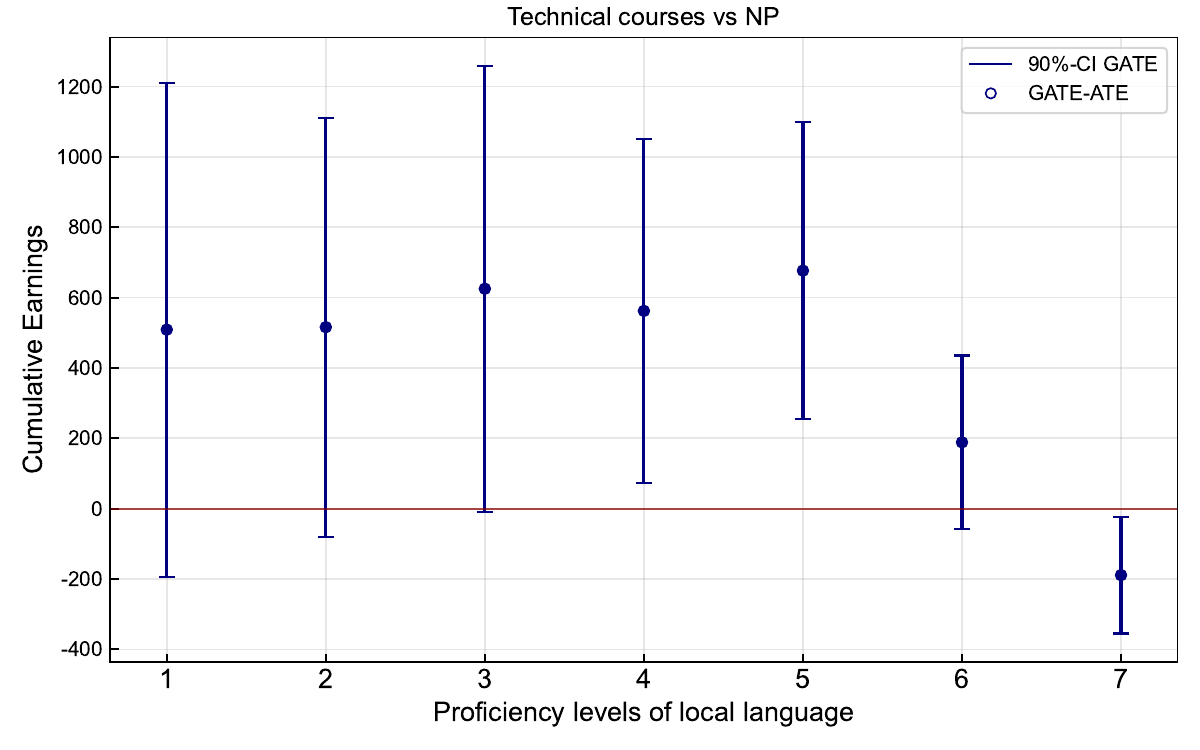}
	\end{minipage}
  \begin{minipage}[t]{0.55\textwidth}
 \includegraphics[width=0.80\textwidth]{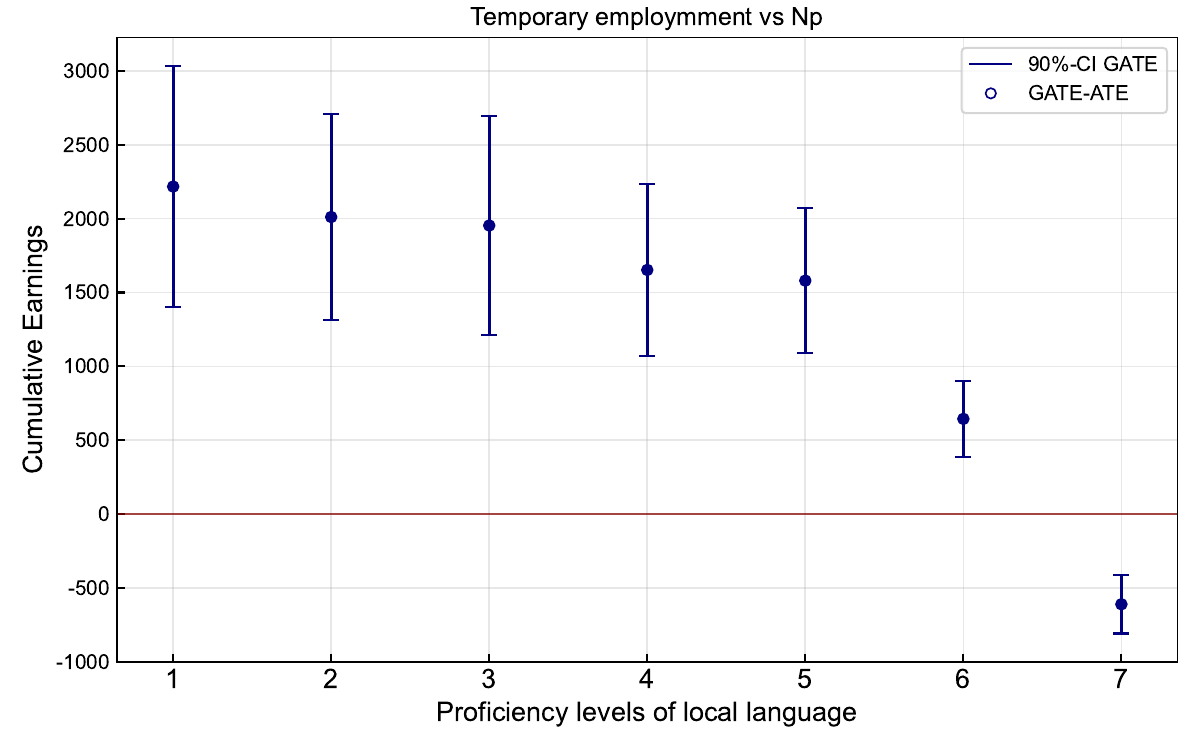}
	\end{minipage}
%Permit type
\begin{minipage}[t]{0.55\textwidth}
 \includegraphics[width=0.80\textwidth]{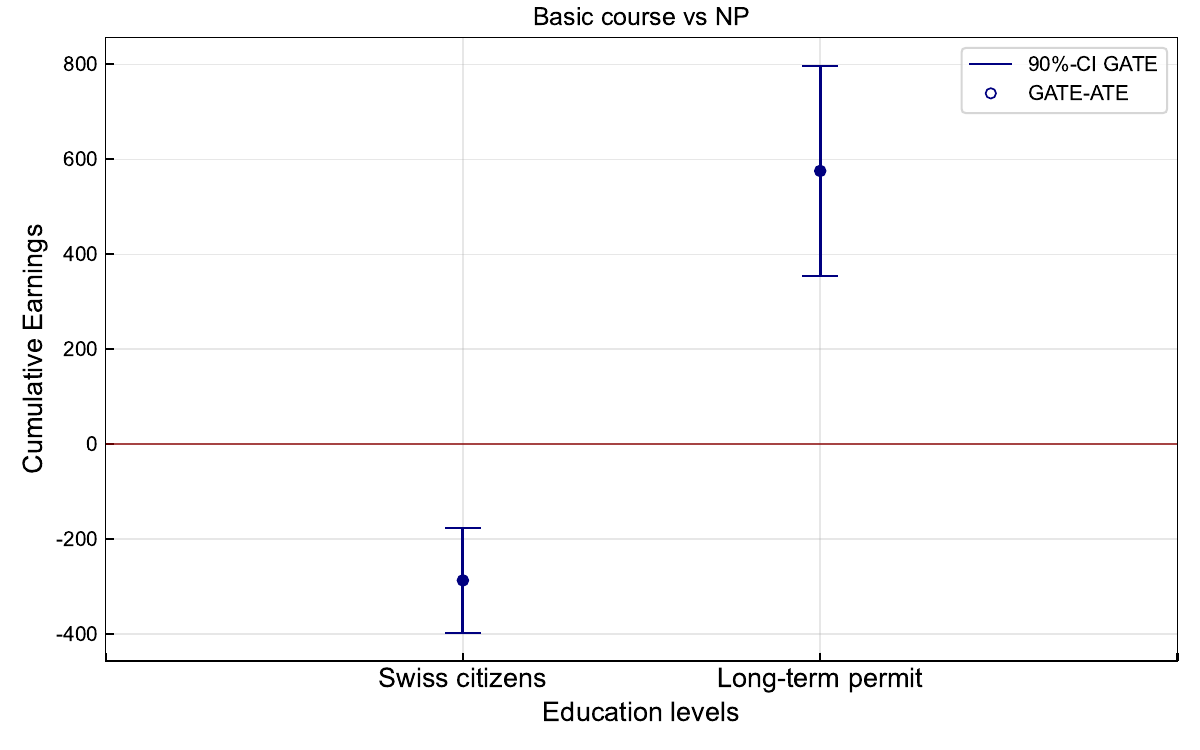}
	\end{minipage}
\begin{minipage}[t]{0.55\textwidth}
 \includegraphics[width=0.80\textwidth]{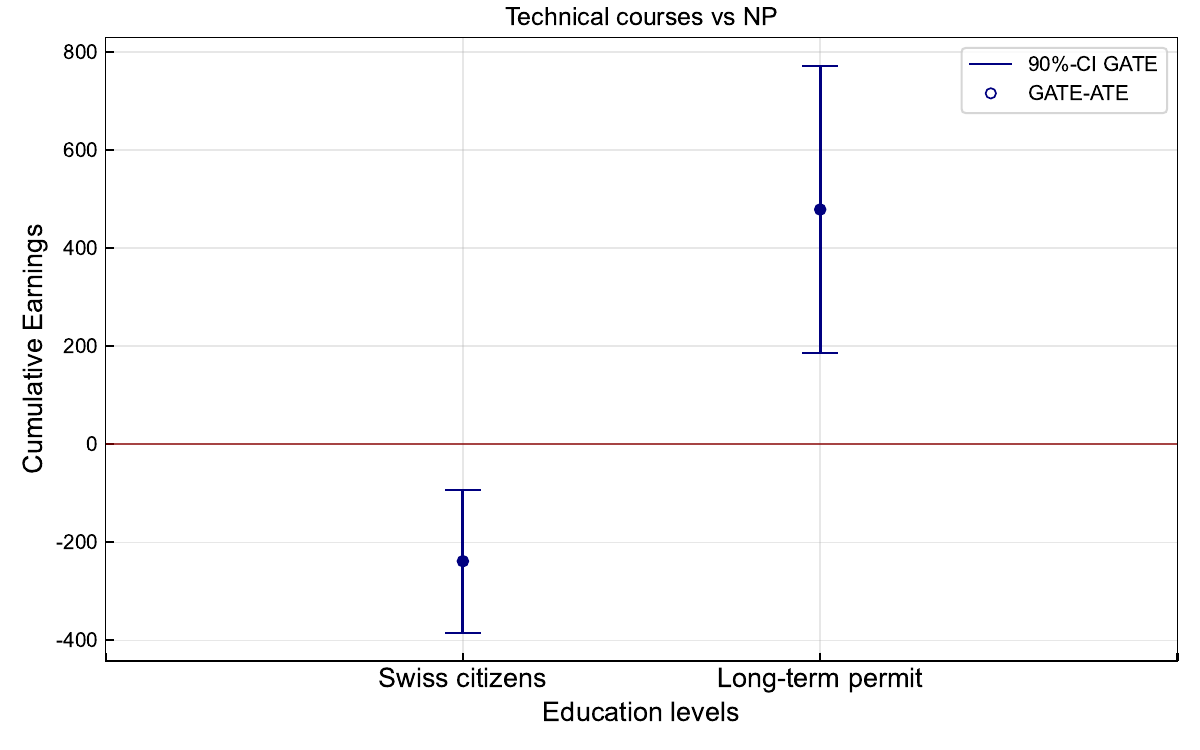}
	\end{minipage}
\begin{minipage}[t]{0.55\textwidth}
 \includegraphics[width=0.80\textwidth]{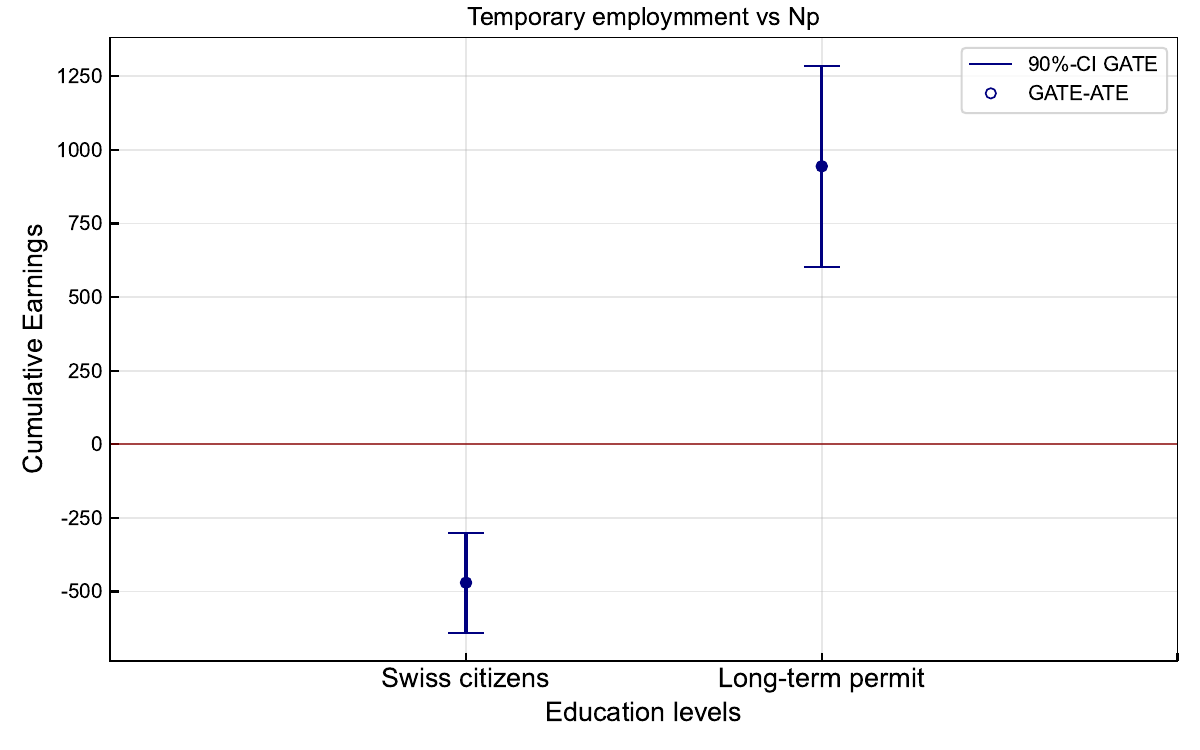}
	\end{minipage}
%Origin
\begin{minipage}[t]{0.55\textwidth}
 \includegraphics[width=0.80\textwidth]{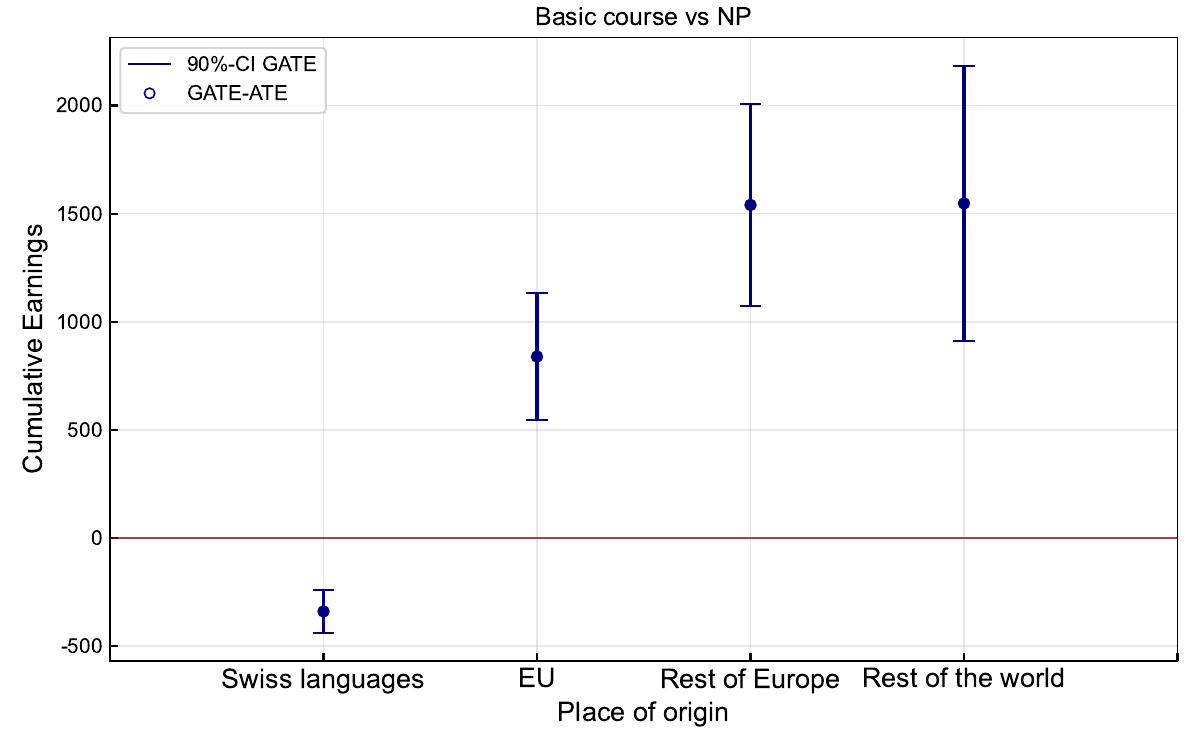}
	\end{minipage}
 
\caption{\textit{Note:} The vertical axes measures the difference of GATEs to the ATE of different programs
with respect to non participants and the 90\% confidence interval. On the horizontal axes the education levels, the proficiency levels in the local language (ordered from the lowest to the highest
levels), the type of permit and the region of origin. The outcome is the cumulative earnings in the third year after the program start.}
\label{fig:gates_appendix}
\end{figure}
