# Supplementary material for: From Average Effects to Targeted Assignment: A Causal Machine Learning Analysis of Swiss Active Labor Market Policies
Source: arXiv:2410.23322 source file (2025-05-11)
Supplement: Supplementary file 3 [file gates_app2.tex]

% GATEs app 
\begin{figure}[H]
\begin{minipage}[t]{0.55\textwidth}
 \includegraphics[width=0.80\textwidth]{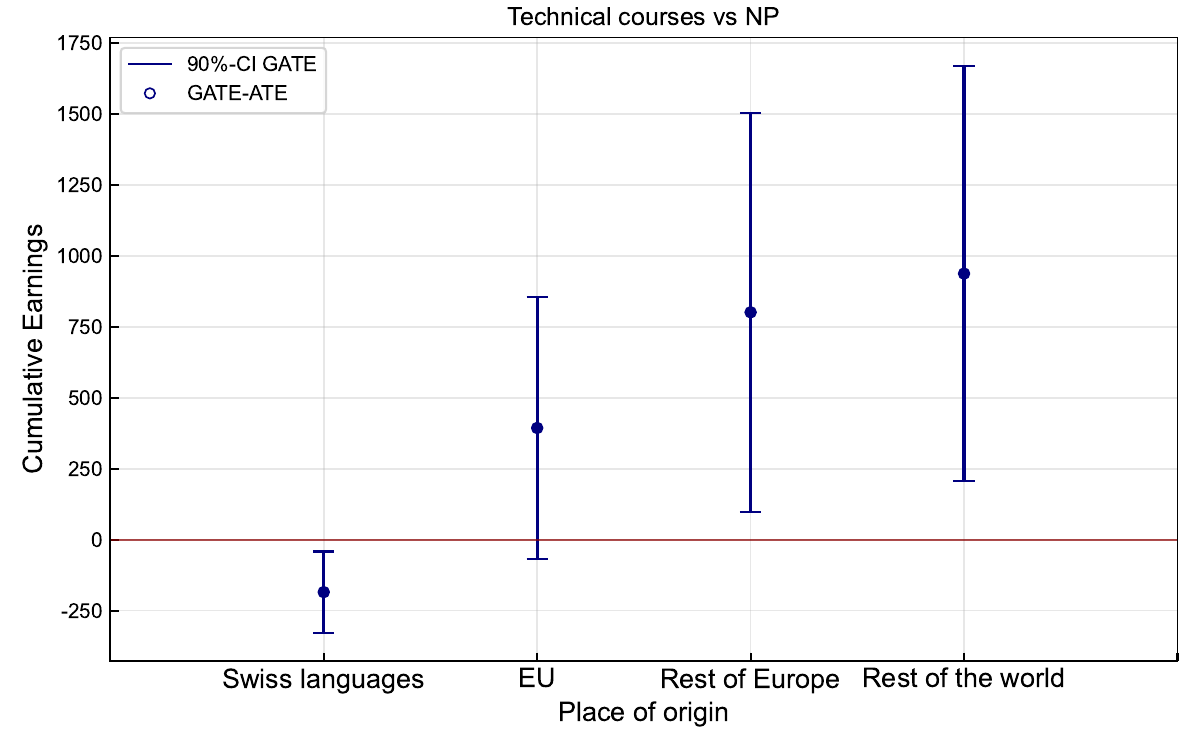}
	\end{minipage}
        \begin{minipage}[t]{0.55\textwidth}
 \includegraphics[width=0.80\textwidth]{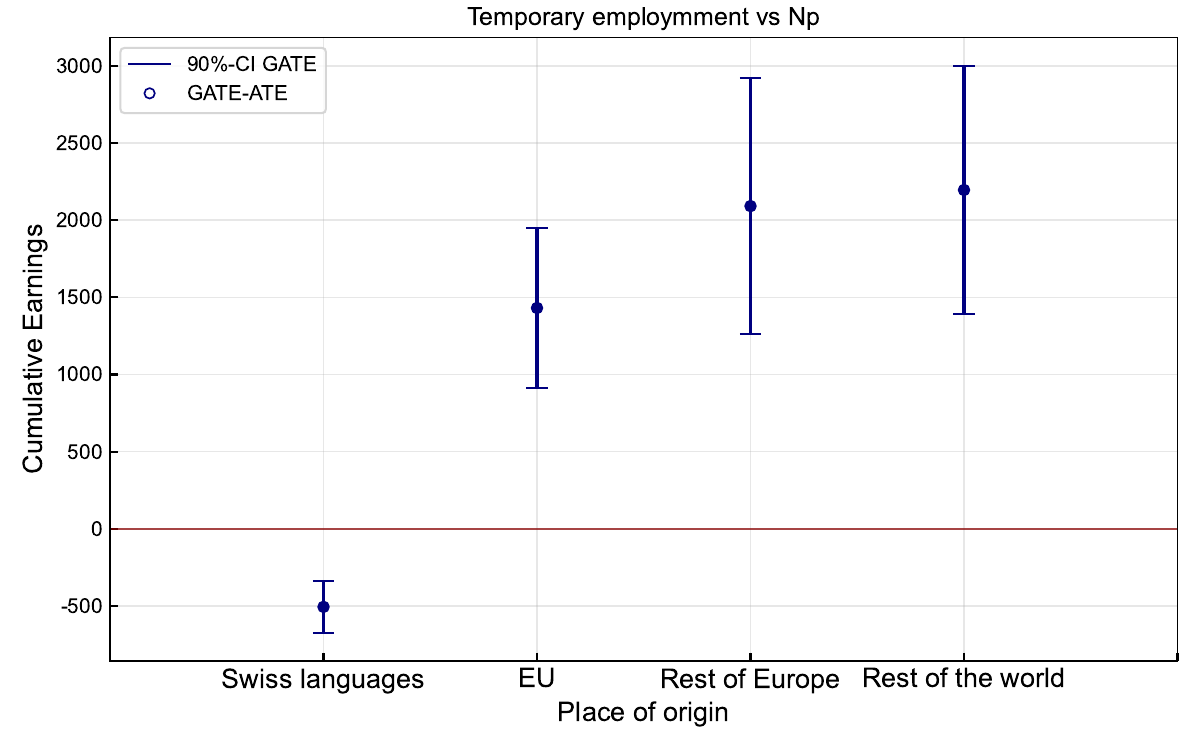}
	\end{minipage}
\begin{minipage}[t]{0.55\textwidth}
 \includegraphics[width=0.80\textwidth]{Plots/GATEs/GATEs_appendix/gate_origin3.pdf}
	\end{minipage}
        \begin{minipage}[t]{0.55\textwidth}
 \includegraphics[width=0.80\textwidth]{Plots/GATEs/GATEs_appendix/gate_origin4.pdf}
	\end{minipage}
\caption{\textit{Note:} The vertical axes measures the difference of GATEs to the ATE of different programs
with respect to non participants and the 90\% confidence interval. On the horizontal axes the region of origin. The outcome is the cumulative earnings in the third year after the program start.}
\label{fig:gates_appendix}
\end{figure}
